# Supplementary material for: Efficient GW calculations via the interpolation of the screened interaction in momentum and frequency space: The case of graphene
Source: arXiv:2304.10810 source file (2023-10-09)
Supplement: Supplementary file 1 [file supporting_information.pdf]

# Efficient GW calculations via the interpolation of the screened interaction in momentum and frequency space: The case of graphene: Supplemental Information

Alberto Guandalini,[1,*] Dario A. Leon,[1,2,†] Pino D'Amico,[1] Claudia Cardoso,[1] Andrea Ferretti,[1] Massimo Rontani,[1] and Daniele Varsano[1]

[1]*S3 Centre, Istituto Nanoscienze, CNR, Via Campi 213/a, Modena (Italy)*
[2]*Department of Mechanical Engineering and Technology Management, Norwegian University of Life Sciences, 1430, Ås (Norway)*

(Dated: October 9, 2023)

## I. SELF-ENERGY INTEGRATION IN ELLIPTIC COORDINATES

As presented in the main text, the rescaled Hartree-Fock self-energy corresponding to the Dirac Hamiltonian for the highest occupied $\pi$ band $v$ of graphene is expressed as:

$$\Sigma'_{vk} = \frac{\gamma_c f}{2\pi} \int \frac{dq_x dq_y}{\sqrt{q_x^2 + q_y^2}} \frac{k - q_x}{\sqrt{(k-q_x)^2 + q_y^2}} \tag{1}$$

where the integration domain is given by $0 \leq q_x^2 + q_y^2 \leq 1$. While polar coordinates are useful to disentangle the integration limits from the variables, as done in the main text, to simplify the expression here we use elliptic coordinates:

$$\begin{aligned} q_x &= \frac{k}{2}(\cosh\mu\cos\nu + 1) \\ q_y &= \frac{k}{2}\sinh\mu\sin\nu \\ dq_x dq_y &= \frac{k^2}{4}(\cosh^2\mu - \cos^2\nu)d\mu d\nu. \end{aligned} \tag{2}$$

with this choice, $\Sigma'_{vk}$ is then expressed as:

$$\Sigma'_{vk} = \frac{\gamma_c f}{2\pi} \int_0^{2\pi} d\nu \int_0^{\mu_m(\nu)} d\mu \, \frac{k}{2}(1 - \cosh\mu\cos\nu), \tag{3}$$

where the upper limit of the integration domain of the second integral is given by

$$\cosh(\mu_m(\nu)) = \frac{2}{k} - \cos\nu. \tag{4}$$

By evaluating the $\mu$ integral in Eq. (3) and substituting $\mu_m(\nu) = \cosh^{-1}(2/k - \cos\nu)$, we obtain

$$\begin{aligned} \Sigma'_{vk} = &\frac{\gamma_c f}{2\pi} \int_0^{2\pi} d\nu \, \frac{1}{2}[k\cosh^{-1}(2/k - \cos\nu) - \\ &\cos\nu\sqrt{4 - k^2 - 4k\cos\nu + k^2\cos^2\nu}]. \end{aligned} \tag{5}$$

Since this integral is still difficult to solve and a numerical treatment results in the Taylor expansions previously discussed in the main text, we will now employ an approximation that allows for an analytical solution.

We note that we have removed the dependence in $\nu$ from the integration domain in Eq. (4) using the following arguments. For any value of $\mu$ and $\nu$, $\cosh\mu \geq 1$ and $-1 \leq \cos\nu \leq 1$, moreover, $2/k \in [2, +\infty]$, therefore $\cos\nu$ is negligible for small $k$. Note that the interdependence between $\mu$ and $\nu$ comes from writing the integration domain, which is a circle, with elliptic coordinates. In Eq. (4), $\cos\nu$ limits ($\pm 1$) correspond to an elliptical domain (see Eq. (2)). As shown in Fig. 1, the lower value, $(\mu_1, \nu_1) = [\cosh^{-1}(2/k - 1), 0]$, corresponds to an ellipse tangent to the original circle at $(q_x, q_y) = (1, 0)$, and with a smaller area (orange); while the larger value, $(\mu_2, \nu_2) = [\cosh^{-1}(2/k + 1), 0]$, corresponds to a larger ellipse, tangent to the circle at $(q_x, q_y) = (-1, 0)$ (blue). It would then be reasonable to approximate the integration domain with an ellipse with

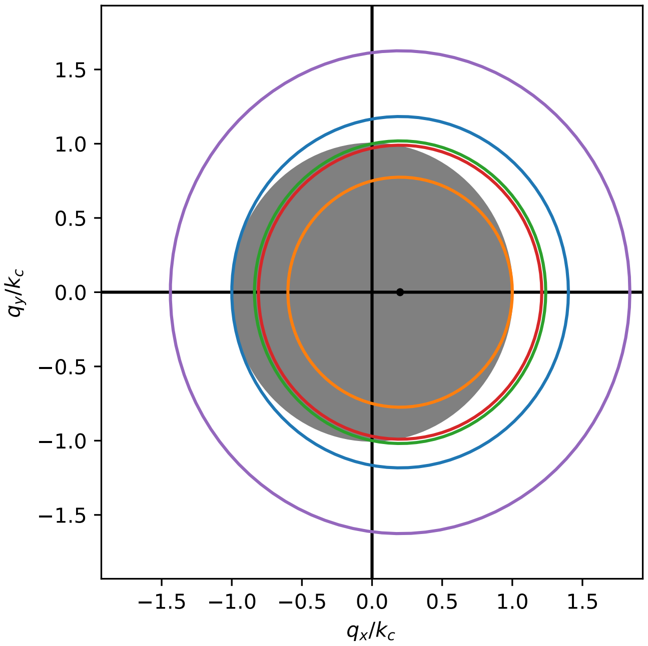


FIG. 1: Integration domains for the exact (Eq. 5) and approximate models (Eq. 6): grey area, exact integration domain; orange line, $\mu_1 = \cosh^{-1}(2/k - 1)$, ellipse tangent to the grey circle at $(q_x, q_y) = (1, 0)$; blue line, $\mu_2 = \cosh^{-1}(2/k + 1)$, ellipse tangent to the grey circle at $(q_x, q_y) = (-1, 0)$; green line, $\mu_s = \sinh^{-1}(2/k)$, which crosses the grey circle in two points close to $(q_x, q_y) = (0, \pm 1)$; red line, ellipse with the same area of the grey circle, i.e, $\mu_a = \sinh^{-1}(8/k^2)/2$; purple line, $\mu_{n=1} = \cosh^{-1}(2/k) + 1/2$. The black dot at $k/2$ set to 0.2 is one of the foci of the ellipses.

$\mu_s = \sinh^{-1}(2/k)$, which crosses the circle in two points close to $(q_x, q_y) = (0, \pm 1)$ (green) or define an ellipse with the same area of the circle, i.e, $\mu_a = \sinh^{-1}(8/k^2)/2$ (red). These two are in fact very similar (green and red lines in Fig. 1). All these four ellipses tend to the same circle in the limit $k \to 0$.

Taking for instance $\mu_m(\nu) \approx \mu_s$, the integral is approximated by an inverse hyperbolic sine:

$$\Sigma'_{vk} \approx \gamma_c f \frac{k}{2} \sinh^{-1}\left(\frac{2}{k}\right). \qquad (6)$$

The first term of the Taylor expansions of these hyperbolic functions around 0 is a logarithmic term, that diverges for $k \to 0$:

$$x \cosh^{-1}\left(\frac{1}{x}\right) = x \log\left(\frac{2}{x}\right) - \frac{1}{4}x^3 - \frac{3}{32}x^5 - O(x^7)$$
$$x \sinh^{-1}\left(\frac{1}{x}\right) = x \log\left(\frac{2}{x}\right) + \frac{1}{4}x^3 - \frac{3}{32}x^5 + O(x^7). \qquad (7)$$

The other terms in the expansions are also similar to those of the exact solution, only a linear term is missing. We can then build simple analytical models based on the hyperbolic functions plus a linear term to approximate the exact solution:

$$\Sigma^n_D(k) = \gamma_c f \left[\frac{k}{2n} \cosh^{-1}\left(\frac{2^{2n-1}}{k^n}\right) + \frac{k}{4}\right]. \qquad (8)$$

Around $k = 0$, $\Sigma^n_D(k)$ has the same Taylor expansion (up to infinite orders) of the exact solution, for any integer exponent $n > 0$. The Taylor expansion for $k \to 1^-$ has the same form:

$$\Sigma^n_D(u \ll 1) = \gamma_c f \left[a^n_0 - a^n_1 u + O(u^2)\right], \qquad (9)$$

where $u \equiv 1 - k$. As mentioned in the main text, the case $n = 1$ is the closest one to the exact solution. Moreover, if we consider a non integer exponent $n = n_0 \approx 0.955327$, we get $a^{n_0}_0 \approx a_0$ (exact solution) and $a^{n_0}_1 \approx 0.310959$. Nevertheless, we find the simpler case $n = 1$ more convenient to use as a fitting model.

In Fig. 1 we have included the elliptic domain that corresponds to $\Sigma^1_D(k)$ (purple). Its size being bigger that the others is a way to compensate for the second term in the parenthesis of Eq. (3), which vanishes when the integration domain, $\mu_m$, is independent of $\nu$.

## II. EFFECT OF THE SMEARING ON GW ENERGIES NEAR THE DIRAC POINT

In this section we discuss the critical role played by the Fermi-Dirac smearing function, which affects the occupations near the Dirac point, and, consequently, the quasi-particle calculations in that region. In Fig. 2 we show the $GW$ band structure of pristine graphene in the region of the Dirac point computed without the use of a smearing function, for three **k**-grids with extra points included with the same method of Ref. [1]. In this scale, the results show no apparent deviation from linearity, with a discontinuity at $K$ slowly closing for denser grids. In fact, the energy difference between $K$ and the closest $k$ point decreases from 0.025 to 0.01 eV when going from a $60 \times 60$ to a $120 \times 120$ **k**-grid. This discontinuity is due to the approximate treatment of the optical limit ($\mathbf{q} \to 0$) in the calculation of the screened interaction and of the self-energy, partially solved by the static $\chi^0_D$ correction described in App. A of the main text.

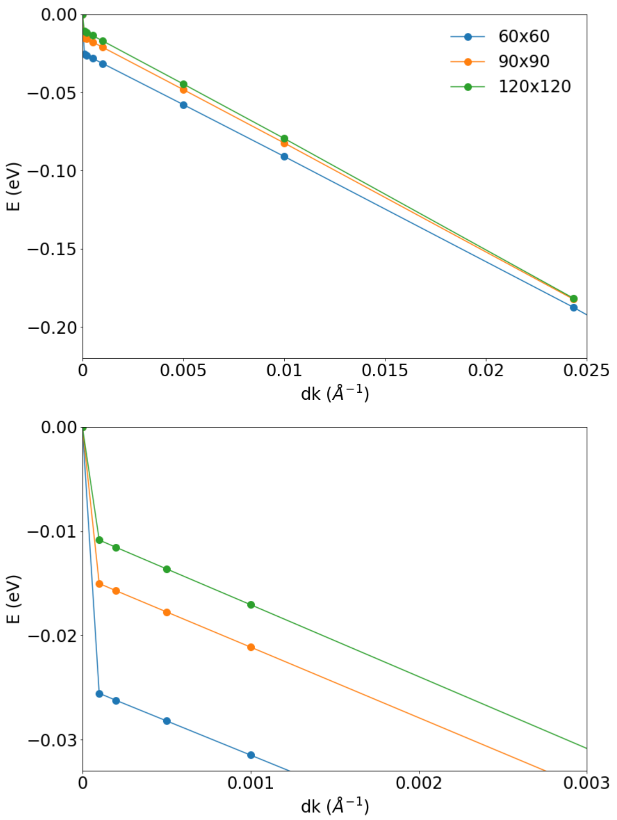


FIG. 2: Graphene valence band in the region close to K, computed with three different **k**-grids and using no smearing.

In order to close the small gap, we use a Fermi Dirac occupation smearing, with a minimum value adjusted to get a smooth dependence for each **k**-grid. A finite smearing is also used in Refs. [1,2]. In Fig. 3 we show the results of applying different values of the smearing to the $60 \times 60$ **k**-grid. The inclusion of a smearing affects the self-energy, modifying the occupations of the states around the Dirac point. Notably, we have included the effects of the smearing in the hyperbolic model presented in the

main text as a $k_s$ shift of the $k$ points in the argument of the $cosh^{-1}$ function.[1]

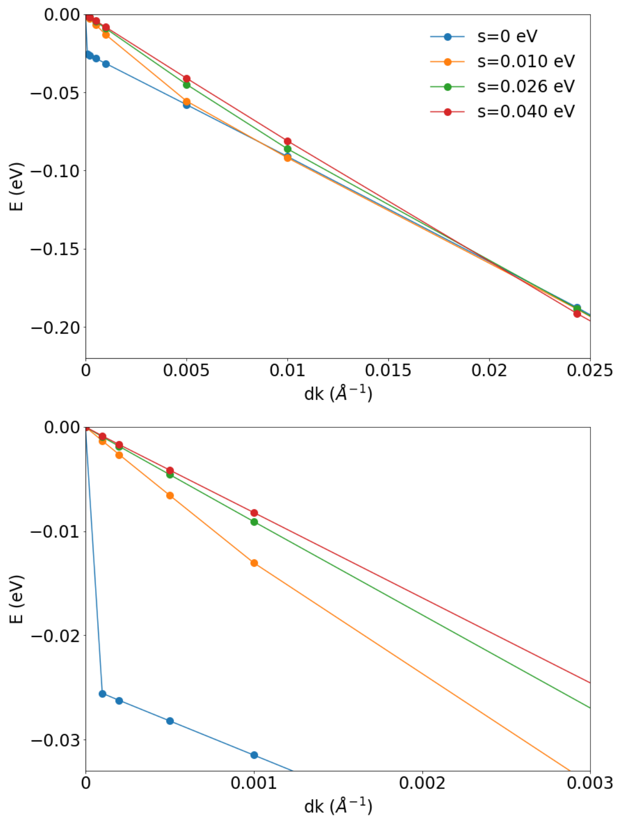


FIG. 3: Graphene valence band in the region close to K, computed with the $60 \times 60$ **k**-grid and using different values of smearing.

Even with the smearing included in the hyperbolic model, different values of the smearing may in principle lead to different fitted parameters, $\gamma_c$ and $f$ (see Eq. (14) in the main text). In order to avoid this dependence, we have performed a series of fits on PPA and MPA calculations with the $60 \times 60$ **k**-grid and different smearing values. As shown in Fig. 4, around $s \sim 30$ meV the standard deviation of the fitted $\gamma_c$ and $f$ parameters is minimal, for both PPA and MPA. A 2D fit simultaneously on $k$ and $s$ spaces confirm the optimal value of smearing for the $60 \times 60$ **k**-grid. In the same figure, we also include the description of the velocity in the linear regime, $\gamma_L$, which also shows a subtle dependence on the smearing. In the main text we show results for the $120 \times 120$ **k**-grid, for which we have used a value of the smearing around half the optimal value found for the $60 \times 60$ **k**-grid.

* Electronic address: alberto.guandalini@uniroma1.it; Current Address: Dipartimento di Fisica, Università di Roma La Sapienza, Piazzale Aldo Moro 5, I-00185 Roma, Italy
† Electronic address: dario.alejandro.leon.valido@nmbu.no
[1] C. Attaccalite and A. Rubio, Physica Status Solidi (b) **246**, 2523 (2009).
[2] P. E. Trevisanutto, C. Giorgetti, L. Reining, M. Ladisa, and V. Olevano, Phys. Rev. Lett. **101**, 226405 (2008).

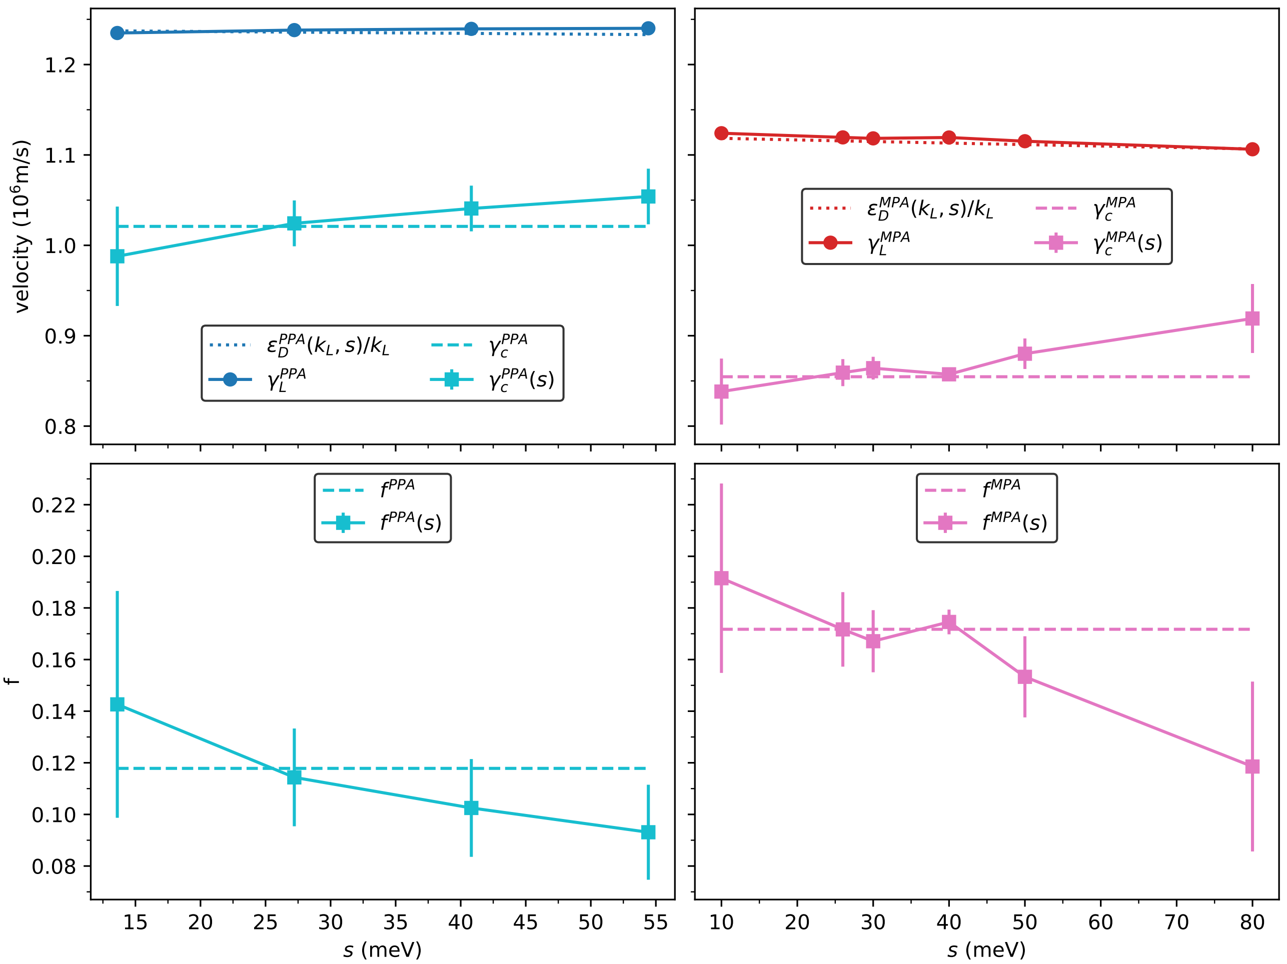


FIG. 4: Velocity (top panels) and $f$ (bottom panels) parameters of the hyperbolic model fitted to the PPA (left panels) and MPA (right panels) results with the $60 \times 60$ **k**-grid. Single points and their errors from all the panels represent a fit with fixed smearing, $s$, while dashed horizontal lines correspond to a 2D fit in $k$ and $s$ spaces with the data of all the smearings. In the case of the velocity, we also include the linear velocity, $\gamma_L$, computed at $k_L = 0.085$ Å$^{-1}$ from the model with both 1D and 2D fits.
